# Supplementary material for: Multiplicative chaos of the Brownian loop soup
Source: arXiv:2107.13340 source file (2022-10-20)
Supplement: Supplementary file 1 [file appendix_details_second_moment.tex]

\section{More details on the proof of Lemma \ref{lem:second_moment_loopmeasure}}

First we fix $z\in D$.
For two independent loops $\Xi^z_{a_1}$ and $\Xi^z_{a_2}$, we also define the multiplicative chaos $\Mc_{a'}^{\Xi^z_{a_1} \cap \Xi_{a_2}^z}$ as follows
\[
\Mc_{a'}^{\Xi^z_{a_1} \cap \Xi_{a_2}^z} :=
\sum_{k,l\geq 1}\dfrac{1}{k! l!}
\sum_{\substack{\wp_1, \dots, \wp_k 
\\ \text{excursions of } \Xi^z_{a_1}
\\ \forall i \neq j, \wp_i \neq \wp_j}} 
\sum_{\substack{\wp_{k+1}, \dots, \wp_{k+l} 
\\ \text{excursions of } \Xi^z_{a_2}
\\ \forall i \neq j, \wp_i \neq \wp_j}} 
\Mc_{a'}^{\wp_1 \cap \dots \cap \wp_{k+l}}.
\]
The intersection measure $\Mc_{a'_1}^{\Xi^z_{a_1}} \cap \Mc_{a_2'}^{\Xi_{a_2}^z}$ is defined similarly by replacing $\Mc_{a'}^{\wp_1 \cap \dots \cap \wp_{k+l}}$ in the above display by $\Mc_{a'_1}^{\wp_1 \cap \wp_l} \cap \Mc_{a_2'}^{\wp_{l+1} \cap \wp_{k+l}}$. One can easily show that the disintegration formula \eqref{eq:disintegration} holds in this context as well:
\[
\Mc_{a'}^{\Xi^z_{a_1} \cap \Xi_{a_2}^z} = \int_0^{a'} \d \alpha' \Mc_{a' - \alpha'}^{\Xi^z_{a_1}} \cap \Mc_{\alpha'}^{\Xi_{a_2}^z}.
\]
Generalisations to higher number of trajectories are immediate.

By the disintegration formula \eqref{eq:disintegration}, the overall thickness $a'$ at $z'$ is evenly spread between the two collections $\{ \Xi_{a_1}^z, \dots, \Xi_{a_l}^z \}$ and $\{ \wp_{l+1}', \dots,  \wp_m \}$. In the computations below, $\alpha'$ (resp. $a'-\alpha'$) denotes the contribution to the thickness $a'$ of the first collection (resp. second collection). $\alpha'$ is therefore uniformly distributed in $(0,a')$ and the left hand side of \eqref{eq:lem_second_moment_loopmeasure} is therefore equal to
\begin{align*}
& \CR(z,D)^a \d z \int_{\mathsf{a} \in E(a,n)} \frac{\d \mathsf{a}}{a_1 \dots a_n} \int_0^{a'} \d \alpha' \\
& \E \Big[ \int \loopmeasure_D(d \wp'_{l+1}) \dots \loopmeasure_D(d \wp'_m) \Mc_{\alpha'}^{\Xi_{a_1}^z \cap \dots \cap \Xi_{a_l}^z} \cap \Mc_{a'-\alpha'}^{\wp_{l+1}' \cap \dots \cap \wp_m}(dz') 
F(z,z', \{ \Xi_{a_i}^z \}_{i=1 \dots n} ; \{ \wp_i' \}_{i=l+1 \dots m} ) \Big].
\end{align*}
By Lemma \ref{lem:first_moment_loopmeasure}, this can be further reduced to
\begin{align}
\label{eq:2p2}
\CR(z,D)^a \d z \int_{\mathsf{a} \in E(a,n)} & \frac{\d \mathsf{a}}{a_1 \dots a_n}
\int_0^{a'} \d \alpha' \CR(z',D)^{a'-\alpha'} \int_{\mathsf{a}'' \in E(a'-\alpha',m-l)} \frac{\d \mathsf{a}''}{a_{l+1}'' \dots a_m''} \\
\nonumber
& \times \E \Big[ \Mc_{\alpha'}^{\Xi_{a_1}^z \cap \dots \cap \Xi_{a_l}^z}(dz')
F(z,z', \{ \Xi_{a_i}^z \}_{i=1 \dots n} ; \{ \Xi_{a_i''}^{z'} \}_{i=l+1 \dots m} ) \Big] 
\end{align}
where all the above loops are independent. By the disintegration formula \eqref{eq:disintegration}, we can decompose
\begin{equation}
\label{eq:2p1}
\Mc_{\alpha'}^{\Xi_{a_1}^z \cap \dots \cap \Xi_{a_l}^z}(dz') = \int_{\mathsf{a}' \in E(\alpha',l)} \d \mathsf{a}' \Mc_{a_1'}^{\Xi_{a_1}^z} \cap \dots \cap \Mc_{a_l'}^{\Xi_{a_l}^z}(dz').
\end{equation}
We now assume that we know that for all bounded admissible measurable function $F'$,
\begin{equation}
\label{eq:2p3}
\Expect{ \Mc_{a'}^{\Xi_a^z}(dz') F'(z',\Xi_a^z) }  = \frac{1}{a'} \CR(z',D)^{a'} \Bs((2\pi)^2 aa' G_D(z,z')^2) \Expect{ F'(z', \Xi_a^z \wedge \Xi_{a'}^{z'} \wedge \Xi_{a,a'}^{z,z'} ) } \d z'
\end{equation}
and we want to argue that it completes the proof. Indeed, by putting this back in \eqref{eq:2p1}, we deduce that
\begin{align*}
& \Expect{ \Mc_{\alpha'}^{\Xi_{a_1}^z \cap \dots \cap \Xi_{a_l}^z}(dz') F''(z', \{ \Xi_{a_i}^z \}_{i=1 \dots l} ) } \\
& = \CR(z',D)^{\alpha'} \d z' \int_{\mathsf{a}' \in E(\alpha',l)} \frac{\d \mathsf{a}'}{a_1' \dots a_l'} \prod_{i=1}^l \Bs ((2\pi)^2 a_i a_i' G_D(z,z')^2) \Expect{ F''(z', \{ \Xi_{a_i}^z \wedge \Xi_{a_i'}^{z'} \wedge \Xi_{a_i,a_i'}^{z,z'} \}_{i =1 \dots l} ) }.
\end{align*}
Coming back to \eqref{eq:2p2}, we have obtained that the left hand side of \eqref{eq:lem_second_moment_loopmeasure} is equal to
\begin{align*}
& \CR(z,D)^a \CR(z',D)^{a'} \d z \d z' \int_{\mathsf{a} \in E(a,n)} \frac{\d \mathsf{a}}{a_1 \dots a_n}
\int_0^{a'} \d \alpha' \int_{\mathsf{a}'' \in E(a'-\alpha',m-l)} \frac{\d \mathsf{a}''}{a_{l+1}'' \dots a_m''}
\int_{\mathsf{a}' \in E(\alpha',l)} \frac{\d \mathsf{a}'}{a_1' \dots a_l'} \\
& \prod_{i=1}^l \Bs ((2\pi)^2 a_i a_i' G_D(z,z')^2) \E \left[ F\Big(z,z',
\{\Xi^{z,z'}_{a_i,a'_i} \wedge \Xi^z_{a_i} \wedge \Xi^{z'}_{a'_i}\}_{i=1}^l ;
\{\Xi^z_{a_{i}}\}_{i=l+1}^n ;
\{\Xi^{z'}_{a''_{i}}\}_{i=l+1}^m \Big)   \right].
\end{align*}
This is precisely the right hand side of \eqref{eq:lem_second_moment_loopmeasure}. Therefore, to conclude the proof of Lemma \ref{lem:second_moment_loopmeasure}, it only remains to show \eqref{eq:2p3}.
